# Supplementary material for: Orbital selective correlations between nesting/scattering/Lifshitz transition and the superconductivity in AFe1-xCoxAs (A=Li, Na)
Source: arXiv:1303.0682 source file (2014-04-29)
Supplement: Supplementary file 1 [file SM.pdf]

# Supplementary information for:
# Orbital selective correlations between nesting/scattering/Lifshitz transition and the superconductivity in $AFe_{1-x}Co_xAs$ (A=Li, Na)

Z. R. Ye,[1] Y. Zhang,[1] M. Xu,[1] Q. Q. Ge,[1] Q. Fan,[1] F. Chen,[1] J. Jiang,[1] P. S. Wang,[2] J. Dai,[2] W. Yu,[2] B. P. Xie,[1,*] and D. L. Feng[1,†]

[1]*State Key Laboratory of Surface Physics, Department of Physics, and Advanced Materials Laboratory, Fudan University, Shanghai 200433, People's Republic of China*

[2]*Department of Physics, Renmin University of China, Beijing 100872, China*

PACS numbers: 74.25.Jb,74.70.-b,79.60.-i,71.20.-b

*Electronic address: bpxie@fudan.edu.cn

†Electronic address: dlfeng@fudan.edu.cn

## I. SAMPLE DESCRIPTION

High quality $LiFe_{1-x}Co_xAs$ [x=0(LiFeAs), 0.03(LC3), 0.09(LC9), 0.12(LC12), 0.17(LC17)] and $NaFe_{1-x}Co_xAs$ [x=0(NaFeAs), 0.045(NC4.5), 0.065(NC6.5), 0.1(NC10), 0.146(NC14.6), 0.32(NC32)] single crystals were synthesized with self-flux method. The starting materials of LiAs (NaAs) and high purity Fe or Co were mixed with 2:1 (4:1) compositions, loaded into an alumina tube, and then sealed into a stainless steel crucible under the Ar atmosphere. The entire assembly was heated to 1323 K (1223 K) and kept for 10 h, and then cooled down to 873 K at the rate of 4 K/h before shutting off the power. Shining platelet crystals as large as $3\times3\times0.05mm^3$ were obtained. The superconducting transition temperatures ($T_C$'s) were ensured by the resistivity measurements with Quantum Design physical property measurement system (PPMS). As shown in Fig. S1(a), for $LiFe_{1-x}Co_xAs$, before the onset of the superconducting transition, the resistivities show clean metallic characteristics without other phase transitions. Superconductivity was observed in LiFeAs, LC3, and LC9 samples with $T_C$ of 16.4, 11, and 4.4 K, respectively. For $NaFe_{1-x}Co_xAs$ [Fig. S1(b)], resistivity anomalies could be observed at 54 K and 43 K in NaFeAs, which are induced by structural transition and magnetic transition respectively [1]. The superconducting transition could be observed at 13, 20.3, 14.8, and 6 K in NaFeAs, NC4.5, NC6.5, and NC10 samples. Note that the drops of the resistivities observed in LC12, LC17, NC14.6, and NC32 might be due to a negligible superconducting volume fraction for these samples.

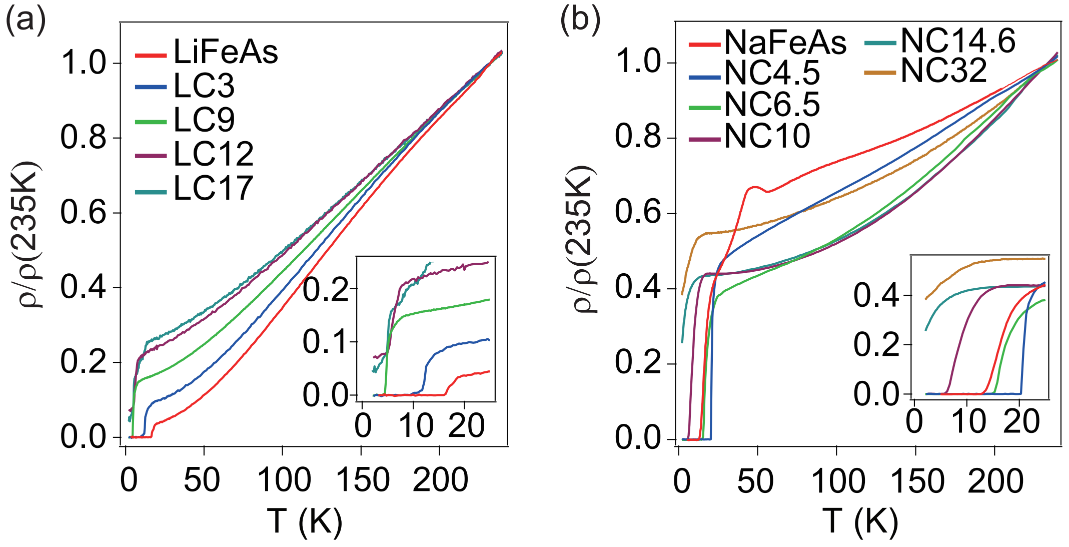


FIG. S1: (a) Temperature dependence of the normalized electrical resistance of $LiFe_{1-x}Co_xAs$. The inset presents the enlarged view of the same data. (b) is the same as (a), but for $NaFe_{1-x}Co_xAs$.

## II. DOPING DEPENDENCE OF THE SUPERCONDUCTING GAP IN $LiFe_{1-x}Co_xAs$ AND $NaFe_{1-x}Co_xAs$

The superconducting gap could be obtained from the symmetrized energy dispersion curves (EDCs) taken at the Fermi crossings (Figs. S2 and S3). The sharp superconducting peaks indicate the high quality of the single crystals. The gap sizes are determined from the fitting process as described in Ref. [2], which are nearly the same as the peak positions as marked in Figs. S2 and S3. The gap size decreases with cobalt doping, as the $T_C$ is suppressed at the same time.

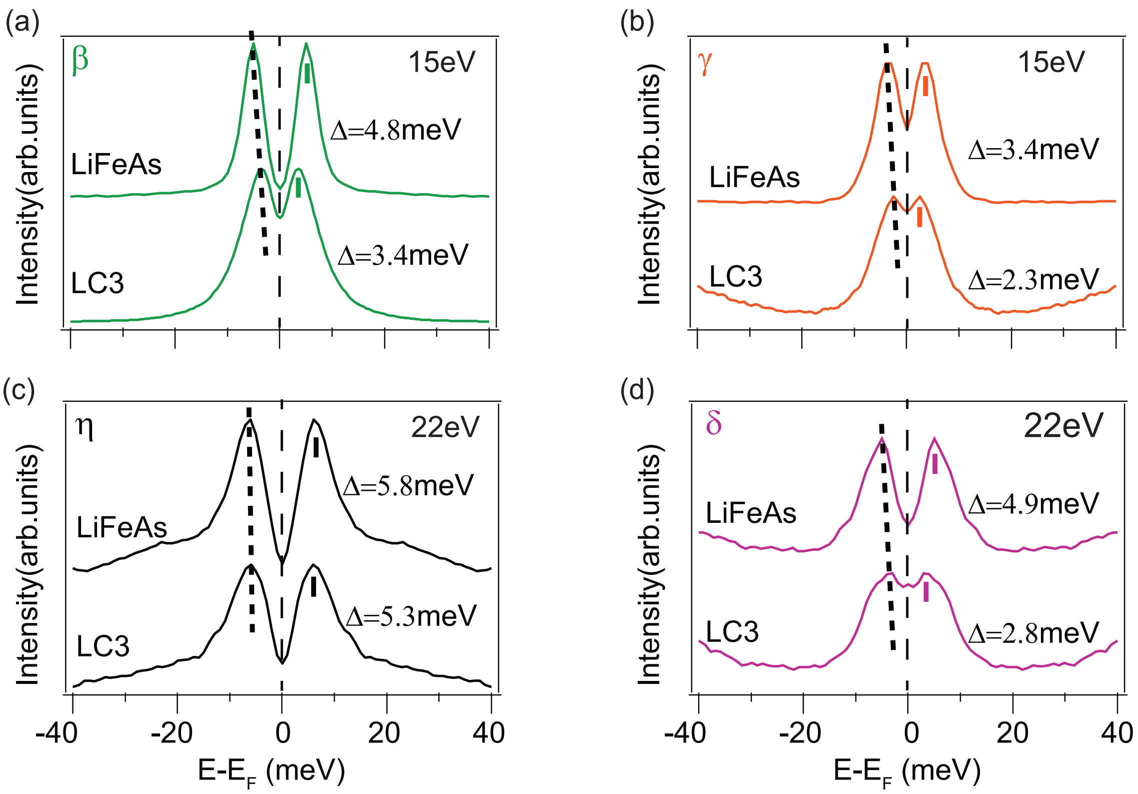


FIG. S2: (a) Doping dependence of the symmetrized EDCs taken at the $k_F$'s of the $\beta$ hole pockets along (0, 0) - ($\pi$, $\pi$) direction in $LiFe_{1-x}Co_xAs$. (b), (c) and (d) are the same as (a), but taken at the $k_F$'s of $\gamma$, $\eta$, and $\delta$ pockets, respectively.

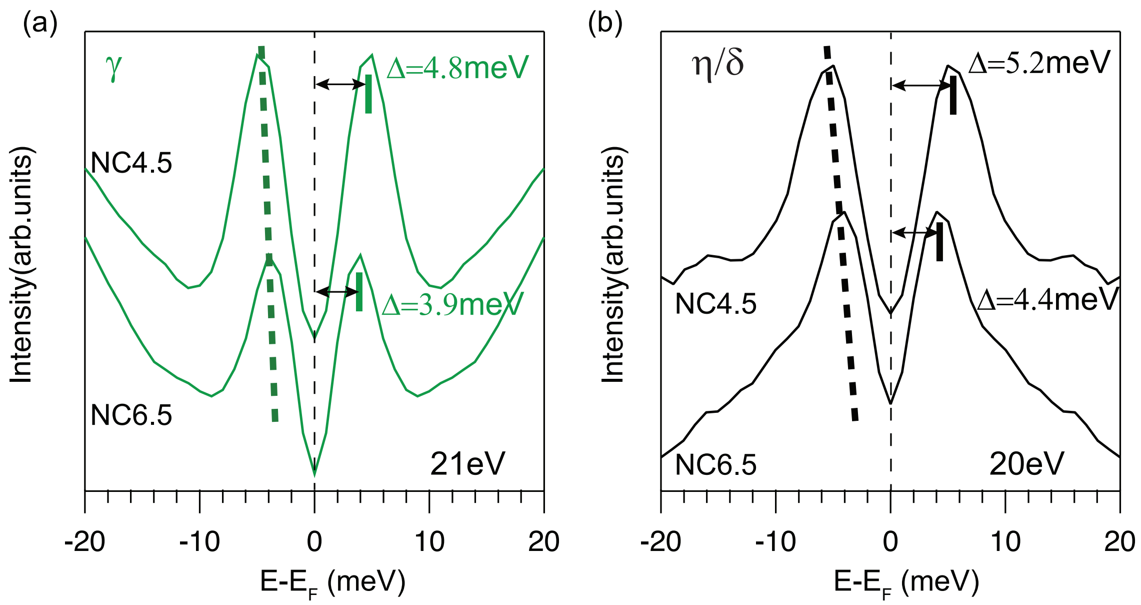


FIG. S3: (a) Doping dependence of the symmetrized EDCs taken at the Fermi crossings ($k_F$'s) of the $\gamma$ hole pockets along (0, 0) - ($\pi$, $\pi$) direction in $NaFe_{1-x}Co_xAs$. (b) is the same as (a), but taken at the $k_F$'s of $\eta/\delta$ electron pockets.

[1] Y. Zhang et al., Phys. Rev. B **85** (8), 085121 (2012).

[2] Y. Zhang et al., Nature Phys. **8** (5), 371-375 (2012).
